# Supplementary material for: The Othello AI Arena: Evaluating Intelligent Systems Through Limited-Time Adaptation to Unseen Boards
Source: arXiv:2508.09292 source file (2025-08-12)
Supplement: Supplementary file 1 [file 96-korean-writeup-supplement.tex]

\section{Intelligent system을 개발하는 과정에서의 주어지는 시간 활용법}

이 숙제를 진행하는 Intelligent system을 숙제로 받은 학생들은 세 단계로 나누어 개발을 할 수 있다.

\subsection{숙제 제출 전까지 충분히 길게 주어지는 1달 정도의 시간인 $T_{\text{Development}}$을 사용하는 방안} 

\begin{itemize}
    \item arena 코드와 API를 철저히 이해하고, 제공된 public stage들을 바탕으로 다양한 실험과 테스트를 진행할 수 있습니다.
    \item 목표는 HW1에 제출했던 최고 성능의 전략보다 더 뛰어난 전략을 생성할 수 있는 지능형 시스템을 개발하는 것입니다. 이 과정을 통해 과제의 의도와 설계 방향을 파악할 수 있을 것입니다.
    \item 3개의 public stage가 제공되며, n개의 hidden stage에서 평가될 것이라는 점을 고려하여, 학생들은 어떤 private stage가 등장할지 고민하고 스스로 추가 stage를 개발(augmented stage)해볼 수 있습니다.
    \item 다만, 3개 이외의 다양한 augmented stage에 대해 모두 좋은 성능을 내는 전략을 생성하는 시스템을 개발하는 식으로만 접근하면 안 됩니다. 이는 AGI를 data interpolation 형태로 개발하는 접근법과 유사하며, hidden stage가 augmented stage와 근본적으로 다를 경우에는 효과적이지 않을 것입니다.
    \item 학생들이 집중해야 할 핵심은 intelligent system이 활용한 stage와 테스트하는 stage가 다른 상황에서, 어떻게 하면 효율적으로 새로운 stage에 적응할 수 있을지를 고민하는 것입니다.
    \item 여기서 더 해보면 좋을 만한 부분은 $T_\text{analysis}$을 어떻게 사용할 지 다각도로 고민하는 것이다. 하단에 작성한 리뷰 1에 대한 대답에서 언급하였듯이, $T_\text{analysis}$의 20\%는 winning condition과 environment dynamics를 을 찾는 데 쓰고, 30\%는 기존 best-performing strategy의 adaptation, 50\%는 몇개의 best-peforming agent간의 self-play를 이용한 parameter fine-tuning에 쓸 수 있다. 이 예제처럼 하고자 하는 것들이 뭔지 정의한 이후에, 각각에 투자할 budget의 비율을 optimize하는 작업은 $T_{\text{analysis}}$에서는 할 수 없는 일이고, 이전 단계인 $T_{\text{development}}$에서 최대한 결정해야 하는 바이다. 

    마찬가지로, 더 하위 단계인 $T_{\text{game}}$을 어떻게 사용할 지 결정을 해야 한다. 8x8 보드에서 게임을 진행할 경우 총 30수를 두어야 끝나는 게임이므로, 대략적으로 10초를 어떻게 활용하는 게 좋을 지 결정을 해 두어야 한다. 이후 adaptation phase에서는 $T_\text{analysis}$
    
\end{itemize}

% \begin{itemize}
    % \item 먼저 숙제 제출 전까지 주어지는 1달 정도 되는 충분한 긴 시간 ($T_{\text{Development}}$)동안, arena 코드 및 API를 이해하고, 주어진 public stage들을 바탕으로 다양한 시도 및 테스트를 해 볼 수 있다. 기존 HW1에 제출했던 최고 성능의 strategy보다 더 나은 strategy를 spawn할 수 있는 intelligent system을 만드는 것을 목표로 하면, 이 과제가 무엇을 함의하고 디자인되었는지 파악해 나갈 수 있을 것이다. 
    % \item 3개의 public stage가 주어져 있고, n개의 hidden stage에 대해 평가할 것이라고 공지를 하였기 때문에, 학생들은 어떤 private stage가 어떤 것이 나올 지 고민해본 후 주어지지 않은 stage를 스스로 개발해본 뒤 (augmented stage), 여기에서도 좋은 성능을 내는 strategy가 뭔지 고민해 볼 수 있을 것이다. 다만 agent (intelligent system)가 주어진 3개 이외의 수많은 augmented stage들을 알고 있는 상태에서, 그 모든 것에 좋은 성능을 낼 수 있는 strategy를 뱉을 수 있는 intelligent system를 짜보는 식으로 이 숙제를 진행을 하면 안 될 것이다. 이거야말로 AGI를 data interpolation 형태로 개발하는 approach이며, hidden stage가 augmented stage와 근본적으로 다를 경우에는 영원히 해결할 수 없을 것이다.     
    % 더불어 이 방법은 적은 environment sample을 가지고 broad generalization을 가능케 하는 이상적인 AGI~\cite{chollet2019ARC}와는 조금 거리가 있다고 생각된다. 
    % \item 숙제가 게시되고부터, 숙제를 제출할 때까지 학생들이 해야 할 일은 intelligent system이 strategy를 만드는 데 사용한 stage와 테스트하는 stage가 다른 상황에서, 어떻게 하면 cost-efficient하게 새로운 stage에 adapt할 수 있을 지에 대한 고민이다.
% \end{itemize}

\subsection{Intelligent system이 새로운 stage를 살펴보라고 주어지는 $T_\text{analysis}$ 시간을 사용법}

Intelligent system이 새로운 stage를 분석하는데 주어지는 시간($T_\text{analysis}$)은 다음과 같이 활용할 수 있습니다:

\begin{itemize}
\item 새로운 문제가 주어졌을 때 가장 먼저 winning condition을 찾아내는 것이 중요합니다. 이를 위해 agent는 자신이 알고 있는 상식을 동원해 게임 내에서 다양한 행동을 시도해봐야 합니다.
\item ValidMoves API는 이러한 이유로 제공됩니다. agent가 어떤 동작을 할 수 있는지 알려주는 것이 디버깅 난이도를 낮추고, 게임 진행을 원활하게 합니다. Model Dynamics를 모르는 상태에서는 게임을 제대로 진행하기 어렵기 때문입니다. 
\item model을 파악한 후에는 각 행동에 대한 reward를 산출해야 합니다.
\end{itemize}
이 접근법은 보드게임 초보자가 웹에서 게임을 하는 것이 실제 카드로 게임하는 것보다 수월하게 배울 수 있는 이유와 유사합니다. 웹 환경에서는 사용자의 턴에 가능한 행동들을 명확하게 보여주기 때문입니다.

\subsection{한 게임을 완료할 때까지 걸리는 시간인 $T_\text{game}$ 사용법}

$T_\text{game}$은 하나의 게임을 완료하는 데 허용된 총 시간 예산을 의미하며, 본 벤치마크에서는 약 10초로 설정되어 있습니다. 이 시간 내에 매 수를 결정해야 하므로, 불렛 체스와 유사하게 단계별로 시간을 배분하고, 가능한 한 프리무브(premove)나 직관 기반 선택을 적극 활용하는 것이 중요합니다~\cite{guga2022time}. 특히, 복잡한 탐색 연산은 최대한 사전 분석 단계에서 처리하고, 게임 실행 단계에서는 미리 학습한 평가 함수를 빠르게 호출하는 방식으로 시간을 절약할 수 있습니다.

\begin{itemize}
  \item Othello 분야의 세계 챔피언급 프로그램은 초단기 시간 제약하에 효율적 탐색 예산 할당 방식을 사용합니다~\cite{othello1982world}.  
  \item Go 및 Othello에 적용된 ‘프로그레시브 시뮬레이션’ 기법은 시뮬레이션 예산을 점진적으로 조정하여 시간 자원을 최적화합니다~\cite{liao2023minizero}.  
\end{itemize}

효과적인 T\_game 사용을 위해 다음과 같은 전략을 권장합니다:
\begin{itemize}
  \item 단계별 시간 할당
    \begin{itemize}
      \item 오프닝: 1수당 0.5–1초 이내로 빠르게 진행  
      \item 중반전: 수급이나 전술적 전환점에서는 1.5–2초, 일반 수에서는 1초 이하  
      \item 종반전: 남은 말의 수와 판 상태에 따라 1초 이내로 결정  
    \end{itemize}
  \item 프리무브(Premove): 가능성이 높은 수를 미리 입력해 두어 시간 소모를 최소화하되, 상대의 의외 수에 대비해 신중히 사용합니다.
  \item 직관적 플레이 및 단순화: 복잡한 탐색 대신, 보드 지형을 몇 가지 핵심 패턴(코너·가장자리 우선 등)으로 단순화하여 빠르게 평가하고 수를 선택합니다.
  \item 사전 계산과 메모이제이션: 미리 계산된 위치 가치 행렬이나 자주 사용되는 수열을 캐시해 두어, 실행 단계에서 즉시 참조할 수 있도록 합니다.
\end{itemize}

이 학생에게(이승필) 오델로를 하게 했음. 알고보니까 이승필 학생은 오델로에 대한 경험은 별로 없었음. 체스는 고수이고, 바둑도 많이 둔 학생인데 오델로는 몇판 안해봄 - 구석이 좋은지 정도만 알고, 구석 먹기 위한 전략 등이 체화되진 않은 레벨 정도 =>  이 오델로 내용을 yinsh 내용 앞에 먼저 써야 할 것 같음. 

3번 stage와 12번 stage에서 이어서 게임을 몇 판 하면서 이야기한 내용과, 완전 새로운 룰인 13번 stage에 대해 게임하는 과정에서 한 질의응답 내용을 직접 적은 것이다. 3번은 c-square 네 곳이 장애물로 막혀있는 보드이고, 12번은 장애물이 있지만 그걸 뛰어넘어서 상대방 말을 
먹을 수 있는 규칙이 하나 더 추가된 보드이다. (= 12번 게임은 3번 게임에 추가 룰이 하나 더 들어감), 13번 stage는 개수가 적은 돌을 가진 사람이 계속 둘 수 있는 stage이다.

\subsubsection{3번 게임을 해본 이후, 보드판은 같은데 장애물의 역할 변동으로 샌드위치 규칙이 변한 12번 게임을 해보면서 한 이야기}

\paragraph{paragraph로 묶는 게 좋으면 paragraph 이름을 줘도 됨 - 이 Paragraph는 - 12번 게임을 진행한 이후에 새로운 stage의 규칙을 파악하는 방법이 무엇이었냐고 묻는 질문에 대한 대답}
일단 도메인 지식들이 있을 것이다. 어떤 상황들이 유리하다는 판단이 있는데, 특정 칸들이 막히거나 보상이 바뀔 때 (downstream task), 이점이라던지 추가되는 정보가 있음. 다운스트림 테스크를 4-5개 보게 되면 이런 게 추가되면 이런게 바뀌겟구나 세부적으로 파악이 될텐데, 방금 히든 stage를 경험하고 나서 느낀 것은, 여기서 좀더 잘하려면 내가 가지고 있는 도메인 지식들 중에서 어떤거랑 가장 비슷했지를 빠른 시간 안에 잘 찾아내는 능력이 필요할 것 같다. 포지션을 잘 파악하고 어디를 차지하는 게 중요할 까 고민해야 하는데, 그거를 빠르게 판단할 수 있는 게 중요해 보인다. 그게 첫번째인 것 같고, 생긴건 3번 게임인데 occlusion ignore 룰이 추가가 된 12번 게임은 1번 게임인 스탠다드랑 비슷할 것 같다는 걸 인지하게 되었고 그걸 파악하고 나니까 이기기에 수월했다.

처음 보는 판을 보고 adjust할 때 내 생각의 흐름은 크게 흐름이 두 가지, 좀 넓게 보면 세가지 같다. 
1. 주어진 상황에서 시뮬레이션을 해봄. 내가 여기 두면 상대가 어디 두겠지 - 이걸 도메인 지식 수준에서 판단을 해보고 아 그러면 이렇게 했을 때 내가 좋아지겠구나, 안좋아지겠구나 직관적으로 판단을 하는 것 같음 (MCTS). 이렇게 생각을 해보니까 이 자리들이 좋아 보이네, 이렇게 좋아지는 점들이 이전에 공부했던 이런 판이랑 비슷하네. (12번째 스탠다드랑 비슷한 것 같다) 이렇게 비교하는 과정을 거친다 - 이게 생각의 흐름.
2. 상대가 둔 수를 보고 판을 평가하려는 것 같기도 함. 상대가 왜 여기 뒀을까 판단하게 되면 좀더 배울수 있는 점이 있는 것 같다. 아까 플레이를 해보니까, 상대를 파악해 보려고 떡수를 둠. 상대가 뭘 두고 싶어하는 지 이해하는 게 포인트임 - 이건 완전전략게임에서 통용되는 이야기라 크게 얻을 건 없었다. 
3. 시각적으로 딱 봤을 때, 이 판이 저번 판과 비슷해 보인다. 룰과는 상관없이 시각적으로 유사하니까 룰도 비슷하겠구나 - 당연한 이야기

리워드 펑션을 빠르게 알수 있어야 되는데, 처음 보는 게임에서는 아무것도 모르는 상태에서 하는 건 어려우니까, 내가 아는 도메인 지식에서 근거해서 알고 있는 지식을 가져와서 적용해보려고 한 것 같다. 

또 승필 학생은 이런 이야기를 함: 정보게임에서는 격언을 많이 씀. 초심자들에게 전달해주고 싶은 격언을 만들곤 함. 중앙을 먼저 잡아라 구석을 먼저 잡아라. 포괄적이고 두루뭉술한 언어로 정보 전달을 받음. 

=> 다른 정보 게임과 뭐가 다르냐면, 처음 보는 상황에서 리워드를 학습해야 하는데, 이런 상황에서 사람들이 주로 취하는 방법은 두루뭉술한 범위에서 언어적인 큰 방향을 도메인 놀리지에 근거해서 어답트를 해오는 것 같음. (룰이 바뀌었을 때 리워드 펑션을 에이전트가 만들려면, 이전에 경험했던 판들과 유사도를 바탕으로 전략을 찾으려고 하는 것 같고, 처음 보는 게임이면 일상적인 표현을 놀리지로 동원해서 전략을 도출해 내려는 것 같음. 어떻게든 경험을 사용해서 리워드를 형성하려는 시도인 것 같음)
 
완전 정보 게임을 처음 배우려는 다른 사람들에게도 이런 현상이 관측되는 것 같다. 리워드가 없는 상황에서 뭔가 배울때에는 도메인 놀리지를 언어의 표현으로 전달하는 것 같다 (모양이 좋다, 기세가 좋다) 말하자면 일상 용어를 판으로 넣는 것 같다, 일상에서 경험한 느낌들을 리워드들을 좀더 어답트하는 데 도움이 되도록 가이드하는 것 같다. 

(내 질문: 바뀐 룰을 관측한 직후, 아차 싶어하면서 전략을 급격히 수정해야 되는 상황을 맞닥뜨리는데, 그때 사람의 thinking process가 key point 일것 같은데). 아까 생각했던 흐름은 비슷하긴 한데, 아 이게 뭐가 달라졌네, 그럼 내가 알고 있는 뭐랑 비슷하지, 그럼 내가 아는 정보 중에서 뭐를 쓸수 있고, 뭐를 쓸수 없지를 고민했던 것 같다. 그래서 이 게임을 끝내자마자 한 생각은 12번 판의 판단기준은 3번보다는 1번 맵의 판단기준과 더 가깝다는 것을 깨달은 것 같다. 그래서 3번 맵에 특화된 전략을 더 사용한 대신 1번 맵 전략으로 수정한 것 같다. - 참고로 이승필 학생은 12번에서 두 판을 둘 수 있었음

사실 맵 모양이 같아서 룰이 바뀌었다는 걸 생각 안하고 뒀었는데,, 만약 1판만 주어지고, 룰이 바뀌었을 거라는 정보를 주고 생각을 하면서 두라고 하면, 처음에는 뭐가 바뀌었는지 탐색을 계속할 것 같다, 바뀐 정보를 파악하고 났을 때, 내가 생각했던 규칙과 달라졌다는 것을 깨달았다면 i.e., 내가 생각했던 판단이 틀렸다는 것을 감지하면 패널티가 더 크게 돌아온다 (감정적인 좌절이 옴). 새로운 룰을 탐색하며 게임을 해야 하다 보니까, specific한 리워드보다는 좀더 보편적인 리워드를 - 손해보지 않으려는 안정적인 접근을 취하면서 탐색을 할 것 같다. 1판 안에 이길 필요가 없다는 걸 이미 알고 있다면, 2판을 해도 된다면(life가 여러 개 있다면), 첫판에는 이것저것 하면서 떡수도 두고 하면서 룰을 파악할 것 같다. exploration은 self-play를 하거나 (안에서 몇 수를 시뮬레이션 해보거나 형세나 위치 판단을 하고), 상대수를 관측하거나 하는 식으로 할 것 같다. (혼자 self-play했을 때 고려하지 않은 수를 상대방이 두면 추가 정보가 생기는 것 같음, 상대가 어떤 걸 가치있게 여기는 지 알 수 있게 된다. 그래서 상대 전략의 강점이나 약점을 분석하는 것 같음. 

상대적으로 고수인 smart-lv-2 agent랑 게임했을 때는 계속 구석이나 변을 최대한 먹으려고 하는구나, 반대로 내가 그걸 먹는 걸 엄청 싫어하는구나를 느꼈음. 돌을 잃더라도 변을 자기가 먹으려는 모습을 보고 그걸 따라하려고 했음. 변을 먹기 위해 돌을 주려는 모습을 계속 봤음.

----
\subsubsection{13번 stage에서 게임을 진행한 후 이야기한 내용}

<한판을 둔 이후 위닝 컨디션을 찾았냐는 질문에 대한 대답>
위닝 컨디션은 똑같다. 시간안에 둘수 있는 곳을 연속해서 둘 수 있는 것이 룰 같음. 내가 빨리 둘 수 있으면 빨리 두는 게 룰인 것 같음 - 이건 재밌는데 - 야 이건 진짜 어렵다. 이건 파악하는 데 어렵다.  

(사실 잘못된 룰을 파악함 = 실제 룰은 현재 판에 상대 돌에 비해 내 돌의 개수가 적으면 몇 번이고 이어서 두는 것임) 빨리 두면 여러번 둘 수 있다라고 룰을 잘못 파악한 상태에서 하는 이야기 -> 생각을 열심히 하는 것보다, 빨리 여러 군데 두어서 턴을 최대한 쓰는 것이 중요해지는 것 같다. 

<불릿 체스에 대해 아는 학생이라 이렇게 물었음, 체스는 그게 중요한 게임일 수 있는데, 오델로도 그게 중요한 게임이냐라는 나의 질문에 대한 대답>  

흠... 고민하더니 "안 잡힐 수 있는 곳에 빨리 많이 두는 게 중요할 것 같다. 그래도 둘 수 있는 데를 단시간에 빨리 두는 게 유리할 것 같다, 어쩄든 한번에 세 수씩 두는 게 - 상대가 한 수 둘 때 세 수두면, 많이 먹히더라도 잡을 기회가 많아지니까 좀더 유리한 것 같다" 라고 했음. 

한판을 더 하더니, "빨리 두는 게 맞는 것 같은데 말한대로 많이 두는게 유리한거 같진 않다. 상대가 오델로를 잘두네." -- 상대했던 전략은 smart-lv-2.js였다. 

몇 판 더 해보았음. (smart-lv-2에서 져서 lv-1을 주고, 그 이후에 greedy를 한 이후에 smart-lv-1를 함)

연속해서 두 번 뒀을 때, 그냥 오델로 판에서는 못이기는 두 수 세 수를 선취해서 먹고 싶은 의표를 찌르겠단 생각을 했고, 그러면 인접한 걸 한번에 두는 게 중요할 수 있겠다는 생각을 했다. (한 area에 여러 번 두어서 특정 영역의 돌을 굳힐 수 있다는 것을 바라본것 같다) 트레이드오프를 했던 것 같다. 너무 막 두면 진다. 시간 안에 여러 번 두지 못하면 내가 둘 수 있는 기회가 사라지니까 생각을 오래하는 대신 빠르게 두어야 함, 내 턴을 뺏기고 상대방이 많이 두게 하면 안될것 같다고 함.

몇 판 둔 뒤에 생각한 룰은 이거였음: 한 수를 둔 이후부터 할당된 시간 동안 여러 수를 둘 수 있음. 상대도 같은 시간 안에 둘 수 있게 되는데, 상대가 먼저 두면 상대 턴이 시작되고, 내가 두 번째 돌을 먼저 두면 다시 세번째 돌을 둘 기회를 상대와 경쟁해서 잡을 수 있음 - 타임어택 게임. 그런 생각을 하면서 최대한 빨리 많이 두려고 했다.  

(결국 룰을 잘못 파악하긴 함 - 판에 있는 돌 개수가 적은 경우에 다음 수를 또 둘 수 있도록 셋업해둔 맵이었는데, 어떨 때는 다음 수를 착수하라는 표시가 연달아 뜨고, 어떨 때는 바로 턴이 넘어가 버린 후 상대가 돌을 둬버리니까 - 또 상대 ai strategy가 빨리 두긴 함, 정확히 룰을 파악하지 못하였음. User Interface과 interaction하는 과정에서 착각을 일으킨 것 같음)
\fi

% 승필과의 오델로 경험을 설명한 글을 주었을 때 Claude의 요약

주요 관찰 내용
1. 오델로 적응 과정 (3번 → 12번 → 13번 스테이지)
3번 → 12번 스테이지 (장애물 규칙 변화)

이승필 학생이 장애물을 넘어서 말을 먹을 수 있는 새로운 규칙을 파악하는 과정
"12번 판의 판단기준은 3번보다는 1번 맵의 판단기준과 더 가깝다"는 통찰
도메인 지식을 활용한 유사성 매칭 (similarity matching)

13번 스테이지 (턴 규칙 변화)

실제 규칙과 다른 잘못된 가설 형성 ("빨리 두면 여러 번 둘 수 있다")
UI 상호작용에서 오는 혼란
불확실한 상황에서의 탐색적 플레이 전략

2. 인간의 적응 메커니즘
사고 과정의 3단계 구조:

시뮬레이션: 내부적 MCTS-like 사고 과정
상대방 행동 분석: 상대의 의도 파악을 통한 학습
시각적 유사성 판단: 보드 모양의 시각적 유사성을 통한 규칙 추론

도메인 지식 활용:

완전정보 게임의 일반적 격언 활용 ("중앙을 먼저 잡아라", "구석을 먼저 잡아라")
언어적 표현을 통한 전략 전달 ("모양이 좋다", "기세가 좋다")

3. 논문에 활용할 수 있는 인사이트
이 대화 내용은 논문의 "Human Adaptation to Novel Board Games" 섹션에 매우 유용한 보강 자료가 될 것 같습니다:

빠른 규칙 발견: 인간이 2-3판 내에 70% 이상의 환경 dynamics를 파악
전이 학습: 기존 게임 경험을 새로운 변형에 적용하는 능력
가설 수정: 잘못된 가설을 형성하더라도 지속적으로 수정해나가는 과정
언어적 추상화: 복잡한 전략을 간단한 언어로 추상화하여 전달하는 능력

이 내용을 통해 AI 시스템이 몇천 번의 시뮬레이션을 통해 달성하는 것을 인간은 훨씬 적은 데이터로 효율적으로 해결하는 과정을 구체적으로 보여줄 수 있을 것 같습니다.
